# Supplementary material for: Unclonable Functional Encryption
Source: arXiv:2410.06029 source file (2025-03-14)
Supplement: Supplementary file 1 [file Appendix2FE.tex]

\section{FE for a family of two circuits}
First we construct daptively secure, single key query, functional encryption for a family of two circuits. 

Let $\mathsf{IdFE} = (\Setup, \Enc, \Keygen, \Dec, \Sim)$ be a classical adaptively secure, single key query functional encryption scheme for the identity circuit. 
Using the classical $\IdFE$ scheme we can construct a quantum FE scheme for the family of two quantum circuits $\mathcal{C} = \{C_0, C_1\}$. 

\begin{itemize}[align=left,leftmargin=2.8em]
    \item[$\bm{\Setup(1^\lambda) \rightarrow (\mpk,\msk)}$] Run the classical $\IdFE$ scheme for $i \in \bin$ to obtain the keys $(\pk_i,\sk_i) \leftarrow \IdFE.\Setup(1^\lambda)$. Output $(\mpk=(\pk_0,\pk_1), \msk=(\sk_0,\sk_1))$ 
    \item \textcolor{red}{[$\bm{\Enc(\mpk, |\phi\rangle) \rightarrow \ct}$]} (Input is a $2$-qubit state?) Take two copies of the input state and create a ciphertext for each circuit. Sample two pairs of keys for the QOTP $(a_0,b_0),(a_1,b_1)$, where $a_i, b_i \in \bin$. Compute $$|\phi_0\rangle = \Xgate^{a_0} \Zgate^{b_0} C_0(|\phi\rangle) \text{ and } |\phi_1\rangle = \Xgate^{a_1}\Zgate^{b_1} C_1(|\phi\rangle).$$ Encrypt the QOTP keys using the classical FE scheme $$\ct_0 = \IdFE.\Enc(\pk_0, (a_0,b_0)) \text{ and }\ct_1 = \IdFE.\Enc(\pk_1, (a_1,b_1)).$$ Output $\ct = (|\phi_0\rangle, |\phi_1\rangle, \ct_0, \ct_1)$. 
    \item[$\bm{\Keygen(\msk, C_b) \rightarrow \sk_b^*}$] Run the $\IdFE$ scheme with  $\sk_b$ as input to obtain the corresponding secret key $\sk_b^* = \IdFE.\Keygen(\sk_b)$.
    \item[$\bm{\Dec(\sk_b^{*}, \ct) \rightarrow |\psi\rangle}$] Given $\ct = (|\phi_0\rangle, |\phi_1\rangle, \ct_0, \ct_1)$ use the key $\sk_b^*$ to obtain the QOPT keys $(a_b,b_b) = \IdFE.\Dec(\sk_b, \ct_b)$ and then decrypt the quantum state $$ |\psi\rangle = \Xgate^{a_b} \Zgate^{b_b} |\phi_b\rangle$$
\end{itemize}

\paragraph{Correctness} Due to correctness of the QOTP and the underlying $\IdFE$ scheme the scheme is correct.

\paragraph{Security}
To show security we construct a simulator $\Sim$ that creates a ciphertext without knowing the plaintext. In the adaptive seurity game the adversary can either first query a secret key and then the ciphertext or first query the ciphertext and then the secret key. 
\begin{enumerate}[align=left, leftmargin=2.8em]
    \item The adversary queries the secret key first. Therefore the simulator obtains the output $C_b(|\phi\rangle)$. The simulator samples keys $(a_0,b_0)$ and $(a_1,b_1)$ and computes: 
    $$|\phi_b\rangle = \Xgate^{a_b} \Zgate^{b_b} C_b(|\phi\rangle) \text{ and } |\phi_{1-b}\rangle = \Xgate^{a_{1-b}}\Zgate^{b_{1-b}} C_{1-b}(|0\rangle)$$

    The classical ciphertexts are computed as in the honest encryption algorithm.
    \item The adversary queries the ciphertext first. The simulator creates two EPR pairs $|\phi_0^+\rangle^{AB}$ and $|\phi_1^+\rangle^{AB}$. The simulator keeps the first qubit of each EPR pair and gives out the second quibt as part of the ciphertext. The classical ciphertexts are simulated via the simulator of the classical FE scheme: 
    $$ \ct_0 = \IdFE.\Sim(\mpk,\emptyset, |x|=2)  \text{ and } \ct_1 = \IdFE.\Sim(\mpk,\emptyset, |x|=2)$$
    The simulator outputs the ciphertext $(|\phi^+_0\rangle^B, |\phi^+_1\rangle^B, \ct_0, \ct_1)$.

    Upon receiving a key query from the adversary the simulator obtains the state $|\phi^{'}\rangle = C_b(|\phi\rangle)$. The simulator uses one of the EPR pairs to teleport the state $|\phi^{'}\rangle$ into the ciphertext. The simulator obtains the teleportation correction keys $(a,b)$ and runs the $\IdFE$ simulator with these keys: 
    $$ \sk_b^* = \IdFE.\Sim(\sk_b, (a,b))$$
    The simulator outputs $\sk_b^*$.
\end{enumerate}

We proof indistinguishability of the real world and the ideal world by a series of Hybrids.

\paragraph{Hybrid 0:} This is the real world, where the ciphertext is created by the Encryption algorithm.

\paragraph{Hybrid 1:} In this Hybrid we use the simulator of the classical $\IdFE$-scheme to simulate the ciphertext in case of an adaptive query. The quantum states $|\phi_0\rangle$, $|\phi_1\rangle$ in the ciphertext are created honestly and the corresponding encryption keys are used to answer the key query using the simulator of the $\IdFE$-scheme. Due to the adaptive security of the $\IdFE$-scheme this change is not noticeable to the adversary. In the non-adaptive case Hybrid 1 remains as Hybrid 0.

\paragraph{Hybrid 2:} This is the Ideal world where the simulator $\Sim$ runs as defined above.
\begin{enumerate}[align=left, leftmargin=2.8em]
    \item Indistinguishability of Hybrid 1 and Hybrid 2 in the case of a non-adaptive query: 
    The only change between Hybrid 1 and Hybrid 2 is the encryption of the state $|0\rangle$ for the part of the ciphertext for which no key was queried. The state is encrypted using a QOTP and the keys of the QOTP are encrypted using the $\IdFE$-scheme. Since the classical $\IdFE$-scheme is CPA-secure the QOTP keys remain hidden and the security of the QOTP applies. 
    \item Indistinguishability of Hybrid 1 and Hybrid 2 in the case of an adapative query: The simulator creates two EPR pairs and sends one qubit each as ciphertexts $|\phi_0\rangle$, $|\phi_1\rangle$. Upon receiving $(|\phi_0\rangle, |\phi_1\rangle, ct_0, ct_1)$ the adversary cannot distinguish this from a ciphertext received in Hybrid 1 since 1 qubit of an EPR pair appears is a maximally mixed state, the same as a state encrypted under the QOTP. $(ct_0, ct_1)$ are ciphertexts simulated by $\IdFE$ as in the previous Hybrid and contain no information about the QOTP keys. 
    Upon receiving the key query the simulator obtains $C_b(|\phi\rangle)$ and teleports the state through the corresponding EPR pair and obtains the correction keys $(a,b)$. The teleported state the adversary now holds is $X^a Z^b C_b(|\phi\rangle)$ which is equivalent to a QOTP encrypted state with the key $(a,b)$, which are revealed using the $\IdFE$ simulator. 
\end{enumerate}
